# Supplementary material for: Can we infer the presence of Differential Privacy in Deep Learning models' weights? Towards more secure Deep Learning
Source: arXiv:2311.11717 source file (2023-11-20)
Supplement: Supplementary file 1 [file appendix.tex]

\section{Full Names for all Methods Reviewed} \label{app:full_names}

This appendix gathers Tables~\ref{tab:app:t1} to~\ref{tab:app:t12}, which list all method reviewed in this study, sorted by their identifier, and giving their full names. Methods named after the initials of their authors' names are marked with the word ``names''. Methods whose name does not refer to neither any acronym nor authors' initials are marked with a hyphen dash (\textbf{``-''}).

\begin{table}[!h]
\centering
\setlength{\tabcolsep}{7pt}

\rowcolors{2}{white}{gray!25}
%\resizebox{\textwidth}{!}{
        \begin{tabular}{C{1cm} L{3cm} L{9cm}}
        \hline
        ID & Acronym & Full Name \\
        \hline
        \input{Tables/Acro/Acronyms_0} \\
        \hline
        \end{tabular}
    %}
\caption{Full names for all methods reviews, sorted by ID (Part I).}
\label{tab:app:t1}
\end{table}

\begin{table}[!h]
\centering
\setlength{\tabcolsep}{7pt}

\rowcolors{2}{white}{gray!25}
%\resizebox{\textwidth}{!}{
        \begin{tabular}{C{1cm} L{3cm} L{9cm}}
        \hline
        ID & Acronym & Full Name \\
        \hline
        \input{Tables/Acro/Acronyms_1} \\
        \hline
        \end{tabular}
    %}
\caption{Full names for all methods reviews, sorted by ID (Part II).}
\label{tab:app:t2}
\end{table}

\begin{table}[!h]
\centering
\setlength{\tabcolsep}{7pt}

\rowcolors{2}{white}{gray!25}
%\resizebox{\textwidth}{!}{
        \begin{tabular}{C{1cm} L{3cm} L{9cm}}
        \hline
        ID & Acronym & Full Name \\
        \hline
        \input{Tables/Acro/Acronyms_2} \\
        \hline
        \end{tabular}
    %}
\caption{Full names for all methods reviews, sorted by ID (Part III).}
\label{tab:app:t3}
\end{table}

\begin{table}[!h]
\centering
\setlength{\tabcolsep}{7pt}

\rowcolors{2}{white}{gray!25}
%\resizebox{\textwidth}{!}{
        \begin{tabular}{C{1cm} L{3cm} L{9cm}}
        \hline
        ID & Acronym & Full Name \\
        \hline
        \input{Tables/Acro/Acronyms_3} \\
        \hline
        \end{tabular}
    %}
\caption{Full names for all methods reviews, sorted by ID (Part IV).}
\label{tab:app:t4}
\end{table}

\begin{table}[!h]
\centering
\setlength{\tabcolsep}{7pt}

\rowcolors{2}{white}{gray!25}
%\resizebox{\textwidth}{!}{
        \begin{tabular}{C{1cm} L{3cm} L{9cm}}
        \hline
        ID & Acronym & Full Name \\
        \hline
        \input{Tables/Acro/Acronyms_4} \\
        \hline
        \end{tabular}
    %}
\caption{Full names for all methods reviews, sorted by ID (Part V).}
\label{tab:app:t5}
\end{table}

\begin{table}[!h]
\centering
\setlength{\tabcolsep}{7pt}

\rowcolors{2}{white}{gray!25}
%\resizebox{\textwidth}{!}{
        \begin{tabular}{C{1cm} L{3cm} L{9cm}}
        \hline
        ID & Acronym & Full Name \\
        \hline
        \input{Tables/Acro/Acronyms_5} \\
        \hline
        \end{tabular}
    %}
\caption{Full names for all methods reviews, sorted by ID (Part VI).}
\label{tab:app:t6}
\end{table}

\begin{table}[!h]
\centering
\setlength{\tabcolsep}{7pt}

\rowcolors{2}{white}{gray!25}
%\resizebox{\textwidth}{!}{
        \begin{tabular}{C{1cm} L{3cm} L{9cm}}
        \hline
        ID & Acronym & Full Name \\
        \hline
        \input{Tables/Acro/Acronyms_6} \\
        \hline
        \end{tabular}
    %}
\caption{Full names for all methods reviews, sorted by ID (Part VII).}
\label{tab:app:t7}
\end{table}

\begin{table}[!h]
\centering
\setlength{\tabcolsep}{7pt}

\rowcolors{2}{white}{gray!25}
%\resizebox{\textwidth}{!}{
        \begin{tabular}{C{1cm} L{3cm} L{9cm}}
        \hline
        ID & Acronym & Full Name \\
        \hline
        \input{Tables/Acro/Acronyms_7} \\
        \hline
        \end{tabular}
    %}
\caption{Full names for all methods reviews, sorted by ID (Part VIII).}
\label{tab:app:t8}
\end{table}

\begin{table}[!h]
\centering
\setlength{\tabcolsep}{7pt}

\rowcolors{2}{white}{gray!25}
%\resizebox{\textwidth}{!}{
        \begin{tabular}{C{1cm} L{3cm} L{9cm}}
        \hline
        ID & Acronym & Full Name \\
        \hline
        \input{Tables/Acro/Acronyms_8} \\
        \hline
        \end{tabular}
    %}
\caption{Full names for all methods reviews, sorted by ID (Part IX).}
\label{tab:app:t9}
\end{table}

\begin{table}[!h]
\centering
\setlength{\tabcolsep}{7pt}

\rowcolors{2}{white}{gray!25}
%\resizebox{\textwidth}{!}{
        \begin{tabular}{C{1cm} L{3cm} L{9cm}}
        \hline
        ID & Acronym & Full Name \\
        \hline
        \input{Tables/Acro/Acronyms_9} \\
        \hline
        \end{tabular}
    %}
\caption{Full names for all methods reviews, sorted by ID (Part X).}
\label{tab:app:t10}
\end{table}

\begin{table}[!h]
\centering
\setlength{\tabcolsep}{7pt}

\rowcolors{2}{white}{gray!25}
%\resizebox{\textwidth}{!}{
        \begin{tabular}{C{1cm} L{3cm} L{9cm}}
        \hline
        ID & Acronym & Full Name \\
        \hline
        \input{Tables/Acro/Acronyms_10} \\
        \hline
        \end{tabular}
    %}
\caption{Full names for all methods reviews, sorted by ID (Part XI).}
\label{tab:app:t11}
\end{table}

\begin{table}[!h]
\centering
\setlength{\tabcolsep}{7pt}

\rowcolors{2}{white}{gray!25}
%\resizebox{\textwidth}{!}{
        \begin{tabular}{C{1cm} L{3cm} L{9cm}}
        \hline
        ID & Acronym & Full Name \\
        \hline
        \input{Tables/Acro/Acronyms_11} \\
        \hline
        \end{tabular}
    %}
\caption{Full names for all methods reviews, sorted by ID (Part XII).}
\label{tab:app:t12}
\end{table}
